# Supplementary material for: Unified Batch Normalization: Identifying and Alleviating the Feature Condensation in Batch Normalization and a Unified Framework
Source: arXiv:2311.15993 source file (2024-03-08)
Supplement: Supplementary file 1 [file fct_supp_imagenet.pdf]

# Res2Net - 50

Before Training

Mid-Training

After Training

BN

Sample index

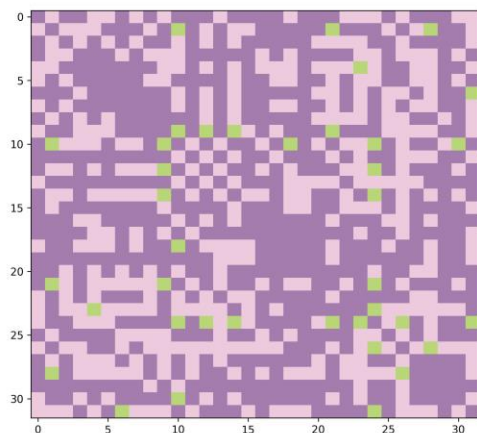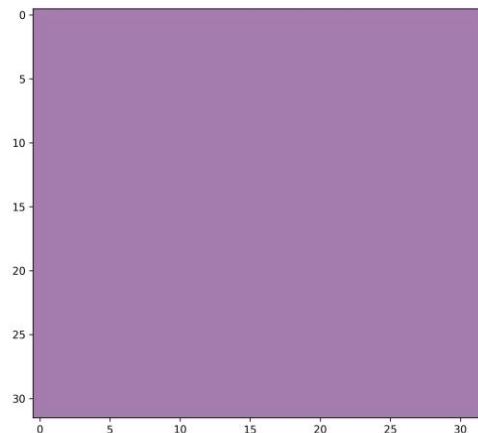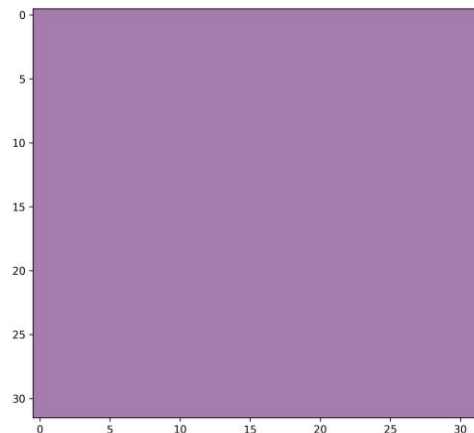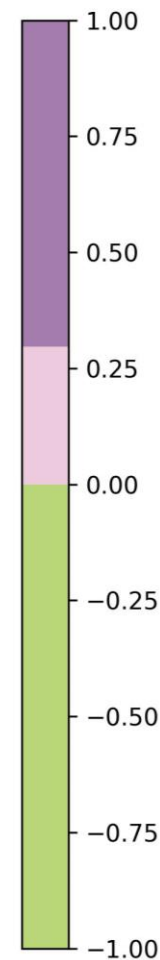

UBN

Sample index

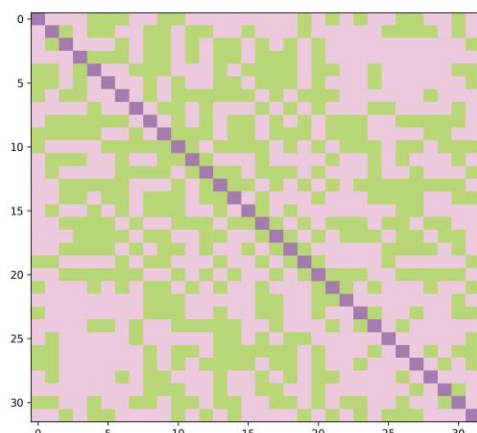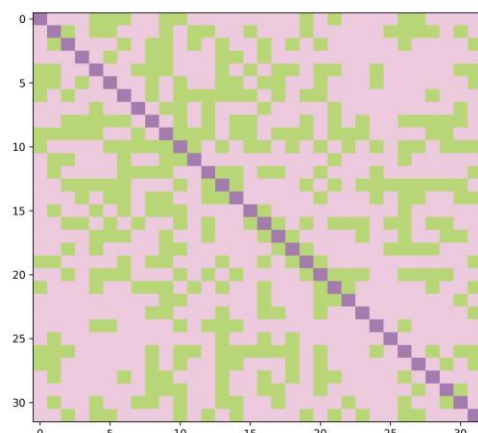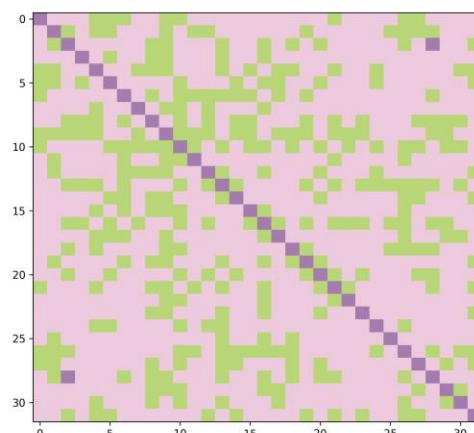

Sample index

Sample index

Sample index

# ResNet-50

Before Training

Mid-Training

After Training

BN

Sample index

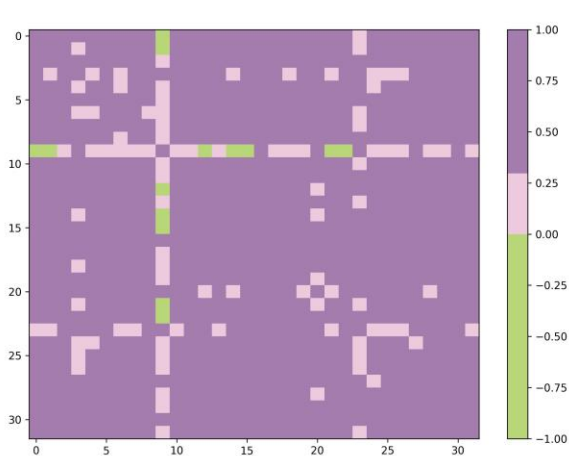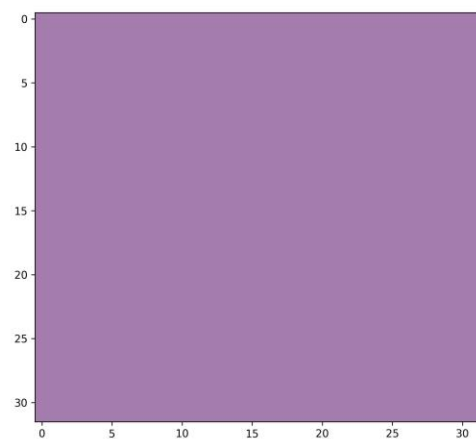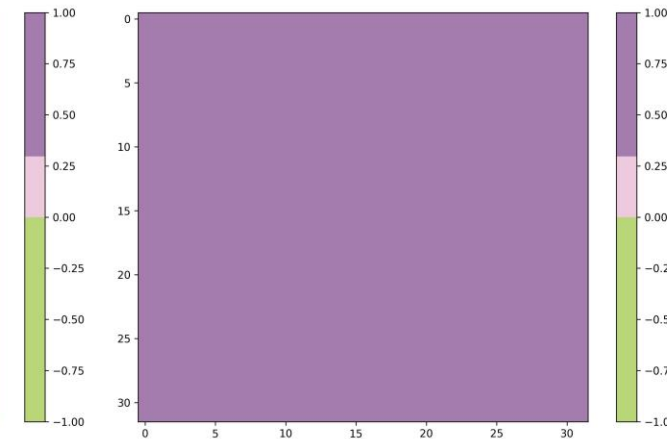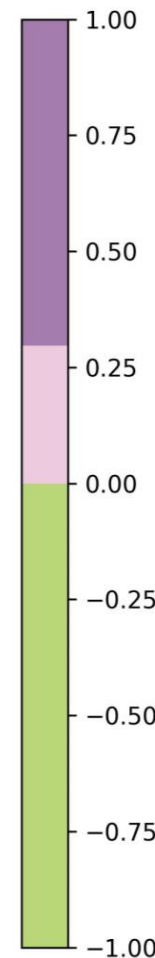

UBN

Sample index

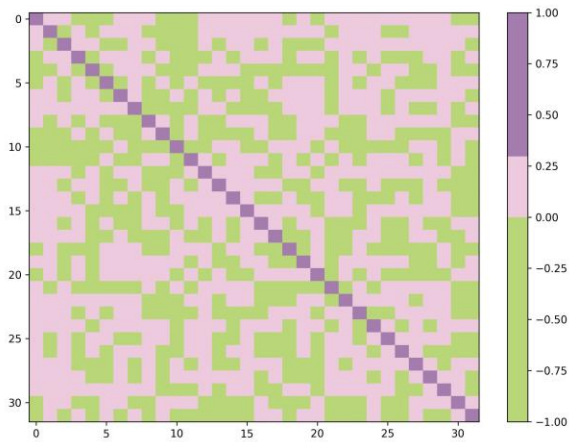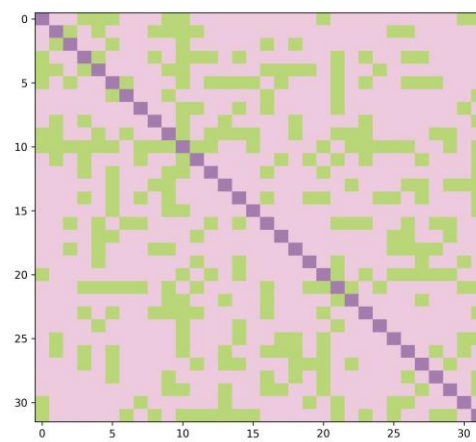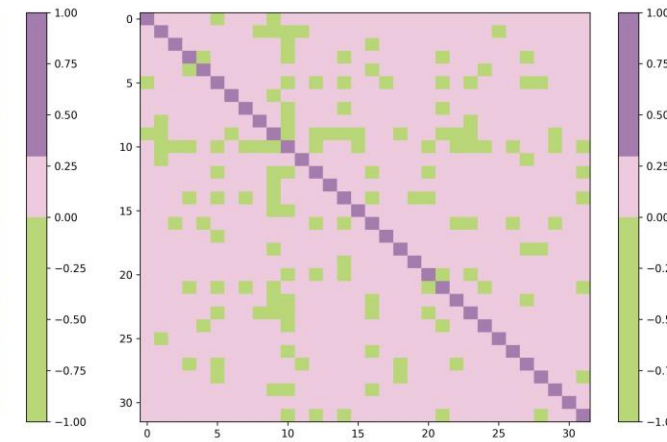

Sample index

Sample index

Sample index

# ResNet-101

## Before Training

## Mid-Training

## After Training

BN

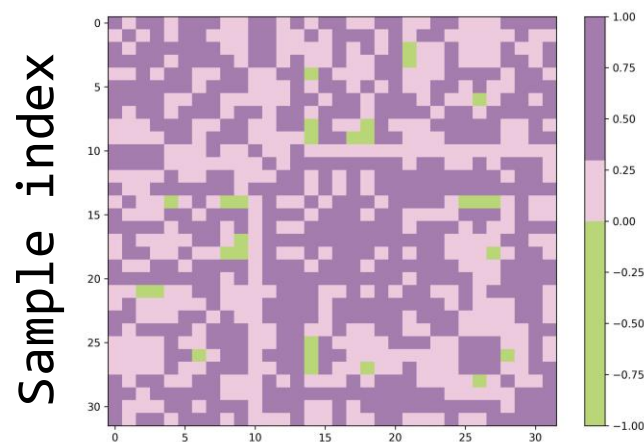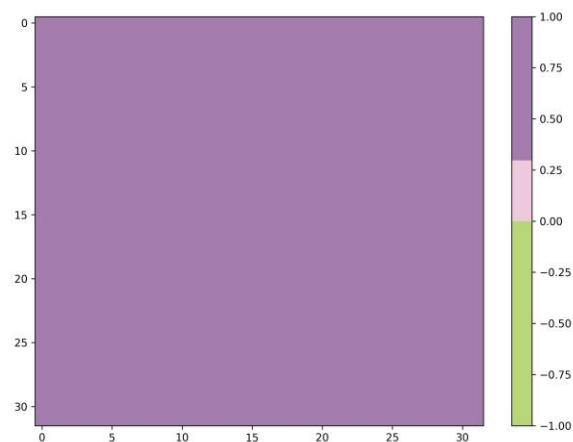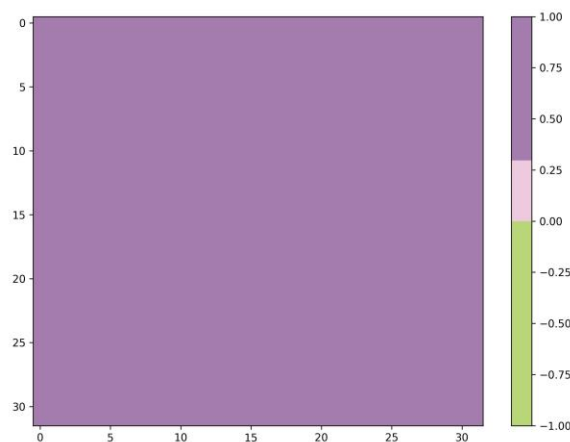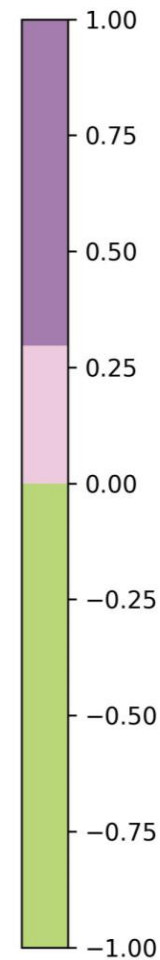

UBN

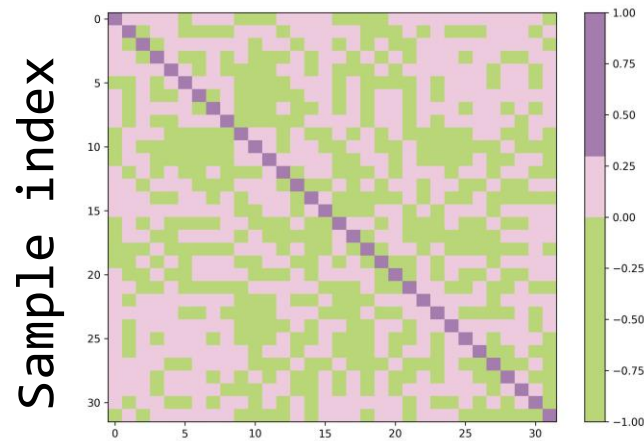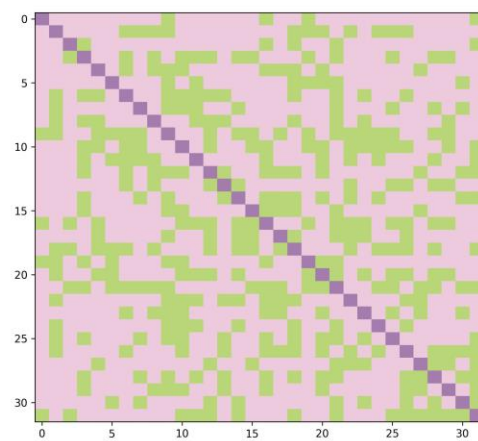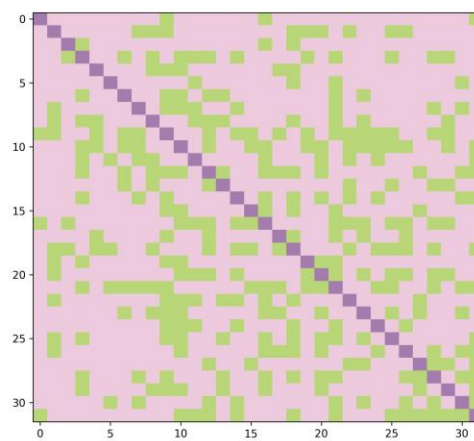

Sample index

Sample index

Sample index

# ResNext-50

## Before Training

## Mid-Training

## After Training

BN

Sample index

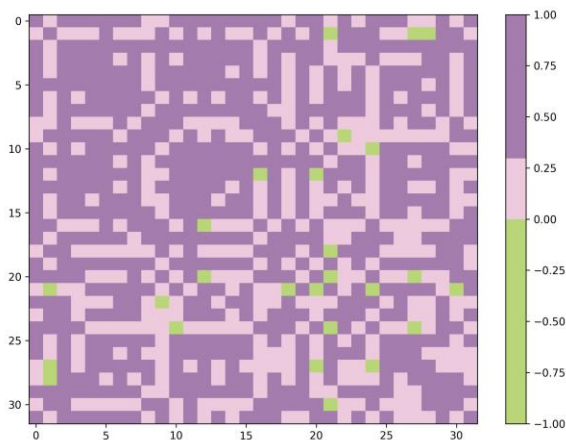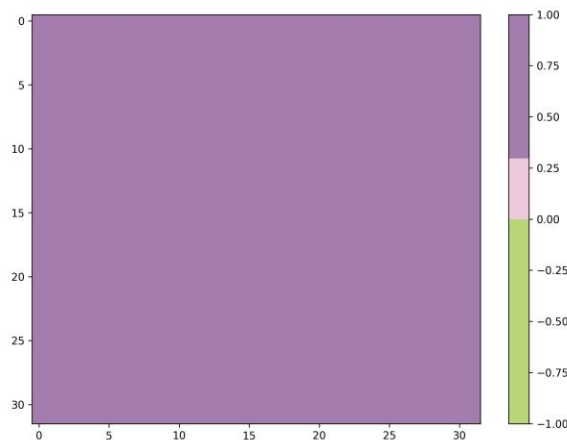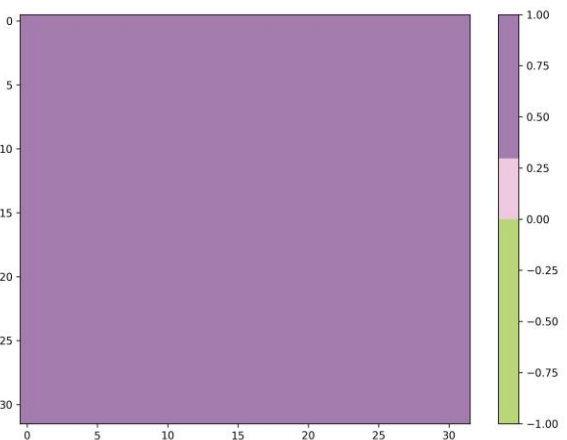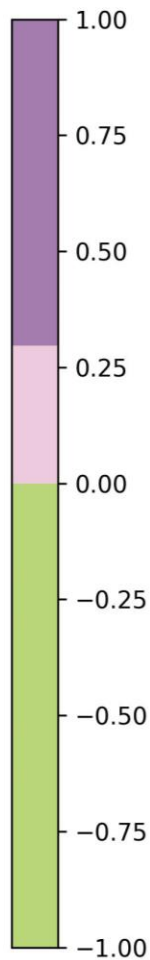

UBN

Sample index

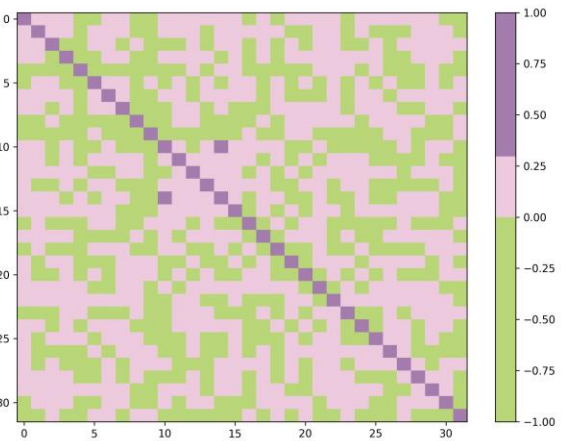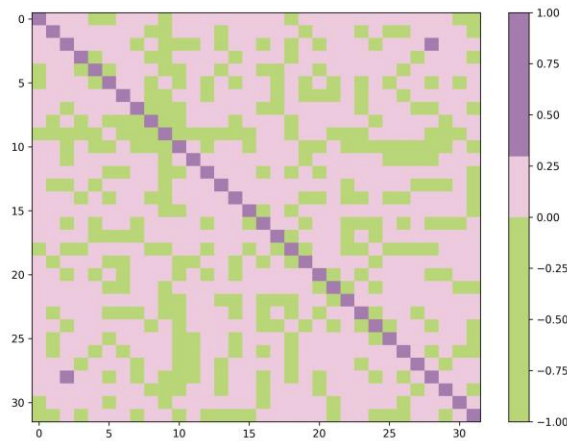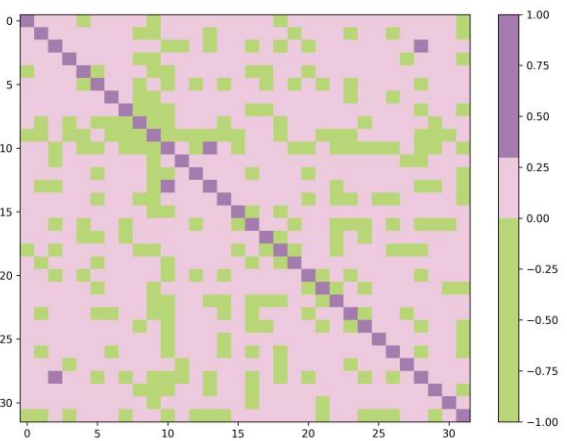

Sample index

Sample index

Sample index
